# Supplementary material for: PNP: Fast Path Ensemble Method for Movie Design
Source: arXiv:1611.02388 source file (2016-11-08)
Supplement: Supplementary file 1 [file 090appendix.tex]

\section{Filtering the data}

On palosgen08: \url{/home/koutrad/GIT_MovieDesign/CODE/PredefinedWalks/SCRIPTS_FOR_DATA}. \\

The mapping to the original names is in:
\url{/home/koutrad/GIT_MovieDesign/CODE/PredefinedWalks/SCRIPTS_FOR_DATA/FeaturesLookup_newDataset_ORIGINAL_NAMES.txt}

\begin{itemize*}
\item Actors: 1-25721  
\item Directors: 25722 - 27043 
\item Producers: 27044 - 31348 
\item Studios: 31349 - 32002 
\item Genres: 32003 - 32029 
\end{itemize*}

\begin{table}[h!]
\centering
\begin{tabular}{l||rrrrr}
Type & Min & Max & Mean & Std & Median \\ \hline \hline
Actors & -6.195 & 8.664 & 0.005 & 0.519 & -0.007  \\ 
Directors & -7.233 & 9.504 & -0.047 & 0.742 & -0.009\\  
Producers & -6.291 & 8.652 & -0.017 & 0.615 & -0.019\\  
Studios & -4.201 & 4.341 & 0.011 & 0.652 & -0.002 \\ 
Genres &  -0.991 & 2.027 & 0.144 & 0.531 & 0.071 \\ \hline
\end{tabular}
\end{table}

The data is under \url{/home/koutrad/GIT_MovieDesign/CODE/PredefinedWalks/REDUCED_DATA}|.\\
\textbf{Filenames}:\\
 F\_thres1\_20\_thres2\_2.mat  \\
R\_thres1\_20\_thres2\_2.mat \\
split\_assignments\_R\_F\_thres1\_20\_thres2\_2

For the sample, we got the best results for:
\begin{itemize*}
\item ALL features (unweighted)
\item original matrix of ratings (without reweighing)
\item feature normalization
\end{itemize*}

\textbf{Lookup for users (old ID, newID)}

{\tt \~/MovieDesign/data/filtered/EDGE\_FILES/MAPPINGS}

\footnotesize{{\tt \~/MovieDesign/data/filtered/EDGE\_FILES/\\
ANON\_user\_profiles\_sex\_location\_age.txt}}

\begin{figure}[h!]
 \includegraphics[width=\columnwidth]{FIG/filtering_data}
 \caption{Process of filtering the data.}
 \end{figure}

 === Different Categories of Users / Target Groups ===\\
 \begin{table}[h!]
 \begin{tabular}{|l|r|}
 adults          &                 14755              \\
 adults 25plus               &          8366              \\
 adults men                   &         5964              \\
 adults women               &           8681              \\
 age18to25                    &          8612             \\ 
 boys                              &     1637              \\
 children                          &     6094              \\
 girls                               &   4403              \\
 men 18to25                   &          3262         \\     
 men 25plus                     &        3483      \\        
 women 18to25                &           5282\\              
 women 25plus                  &         4833                                
\end{tabular}
 \end{table}

\section{Discussion with Christos}

\reminder{
\begin{problem}[Movie Design]
The problem can be generalized in the following way:
\begin{itemize}
\item Given: 
\begin{itemize} 
\item a set of users $\mathcal{U}$, 
\item their preferences $\matR$ ($u x m$ matrix, with entries $r_{ij}$), and 
\item movie features $\matF$ ($m x f$ matrix, with entries $f_{ij}$) 
\item the social network of the users in $\mathcal{U}$
\end{itemize}
\item Find:   how can we design a movie \textbf{within
            budget} that will maximize the influence propagation
            on the given subnetwork of users?
\end{itemize}
\label{prob:influence}
\end{problem}
}

\begin{itemize}
\item Related Work: How to find dependencies in data
\begin{enumerate}
\item SPAM detection based on common terms (Naive Bayes)
\item Pedro Olmo (basketball, KDD '08)
\item Bioinformatics
\end{enumerate}
\item Maximize the rating/adoption across a subset of users
\item Next meeting: Tue 5th, @1pm

\item Tri-partite -> bi-partite to learn weights on edges between users and features: 
a) Belief propagation
b) Random walk with restarts
c) Katz distance
d) Naive Bayes

\item Conversion models: 
a) Threshold based
b) Binarized
c) Random walk from features to get probabilities on the users
Compare these with cross-validation

Optimization Problem: 
a) Budget constraint
b) Cardinality constraint
c) Other types of constraints (later)

Look at Pipage Rounding technique by Ageev et al.

\end{itemize}

\paragraph{Potential Formulation 2: Graph Problem}

\textbf{Heavy-weight subgraphs with color constraints and budget.} We can create a heterogeneous network with all the movie features (e.g., actors, directors, production companies, genre), and link two features if they contributed to the same movie. The edge weight can be a function of the times the two features appeared in a movie, as well as the taste of the target audience. Assume that we can find the user ratings for individual features, $r_{f_{ij}}$ (or the probability that each user likes a feature). Then, we can find a {\it good summary / aggregate} of the individual features, and (a) use it as a node attribute, or (b) convert it to an edge attribute. Moreover, each node needs to be associated with a color which describes the type of feature, and a cost, $c_j$.

\textbf{Dependencies.} If we have dependencies, like an actor working only for a specific production company, we can set the weight of the edge that connects the two entities to a large value.

\textbf{Constraints.} If there are pairs of features that should not appear in the same movie, we can set the corresponding edge weight to a large {\it negative} value.

If we formulate the problem this way, then we are after the heaviest weight subgraph that satisfies the color constraints (e.g., at least one director, actor), and has total cost, $C=\sum_j{c_j}$ smaller than the budget $B$.
\reminder{We need to think how to bring the users in the graph. Maybe link the users to the features of the movies they've rated, and require to maximize the number of people that are adjacent to selected features?}

\textbf{Work on heavy-weight subgraphs.} 
In \cite{BogdanovFMPRS13} the aim is to find contiguous anomalous regions in a weighted dynamic network. The proposed algorithm takes as input timestamps of a weighted graph, where the edge weights represent their anomalous score. The Heaviest Dynamic Subgraph is related to the problem they study, 
and two instances of that are: (a) Maximum Subsequence, and (b) Heaviest Subgraph \cite{BogdanovMS11}.

In \cite{RanuS09}, Ranu and Singh propose an algorithm to find significant subgraphs in large graph databases (reminds me of apriori for graph structures).

\subsection{Data}

\begin{itemize*}
\item 23,776 movies have been rated by at least 5 users
\item 66,726 total flixster movies
\item 83,017 total mgo movies	
\item 17,307 movies both in flixster and mgo (with multiple ids for the same movie)
\item After merging mgo and flixster and collapsing the movie ids that correspond to the same movie: 13,184 movies

\begin{table}[h!]
 \begin{tabular}{ l | c }
   Number of movies & mgo\_IDs \\ \hline
   10760 & 1 \\
   1529 & 2 \\
    498 & 3 \\
    213 & 4 \\
     87 & 5 \\
     43 & 6 \\
     27 & 7 \\
     10 & 8 \\
      8 & 9 \\
      5 & 10 \\
      3 & 11 \\
      2 & 12 \\
  \end{tabular}
\end{table}

\item Multiple movies with same name: 2,425
<<<<<<< HEAD
\item Number of movies to fetch details for 10760
\item Total movies with details: 10,760
\item Total movies with something wrong 0
\item Total features (binarized): 279,054
\item 242,598 edgeFile\_movie\_actors.txt
\item 1,762 edgeFile\_movie\_directors.txt
\item 28,965 edgeFile\_movie\_producers.txt
\item 3,092 edgeFile\_movie\_studios.txt
\item 2,637 edgeFile\_movie\_genre.txt
\item 4,793,786 (before removing dups 7,960,039) movies\_users\_ratings.txt
\item idx 1 - 140,801: actors (140,801 actors)
\item idx 140,802 - 142,114: directors ( directors)
\item idx 142,115 - 156,396: producers ( producers)
\item idx 156,397 - 158,035: studios ( studios)
\item idx 158,036 - 158,060: genres ( genres)
=======
\item Number of movies to fetch details for 10,760
\item Total movies with details: 10,760
\item Total movies with something wrong 0
\item 324,520 Total number of movie-feature edges
\item 253182 edgeFile\_movie\_actors.txt
\item 12,330 edgeFile\_movie\_directors.txt
\item 38,071 edgeFile\_movie\_producers.txt
\item 7,553 edgeFile\_movie\_studios.txt
\item 13,384 edgeFile\_movie\_genre.txt
\item 4,793,786 (before removing dups 7,960,039) movies\_users\_ratings.txt
\item idx 1 - 146,965: actors (146,965 actors)
\item idx 146,966 - 153,468: directors (directors)
\item idx 153,469 - 172,062: producers (producers)
\item idx 172,063 - 174,959: studios (studios)
\item idx 174,960 - 174,986: genres (genres)
>>>>>>> ee8819a717539cf72d5a6ab554e1141fe1c9fc7d
\end{itemize*}
